# Supplementary material for: OpinionConv: Conversational Product Search with Grounded Opinions
Source: arXiv:2308.04226 source file (2023-08-08)
Supplement: Supplementary file 1 [file SIGdial23-opinionConv-part10-appendix.tex]

\onecolumn
\appendix
\newpage
\section{Conversation Templates}

\textbf{Conversation Template ID: 1}

\begin{table}[H]
\centering
\small

\begin{tabular}{@{}p{3cm}p{8.75cm}@{}}
\toprule
\bfseries Pair & \bfseries Example \\
\midrule
Request--Inform &
{\bfseries C:} Can you give me your thoughts on its camera quality? \\
& \textcolor{salesassistantblue}{{\bfseries S:} I did take several pictures and a bit of video with the camera and I was very impressed with the quality.} \\
\midrule
Deny--Disagreement &
{\bfseries C:} As far as I know about its battery, it has no replaceable battery which is a deal killer for me. \\
& \textcolor{salesassistantblue}{{\bfseries S:} I understand your concern, but the original battery life really impress me so you don't need to worry about this issue.} \\
\midrule
Request--Inform &
{\bfseries C:} Ah! I see! What is your opinion about its hardware? \\
& \textcolor{salesassistantblue}{{\bfseries S:} I bought this phone for myself and even with its one year old dated hardware, it still runs as fast as the newest android phone, because the company cares and has complete control over its OS so that it can be optimized the high extent.} \\
\bottomrule
\end{tabular}
\caption{A dialogue example of conversation template (ID:1) in dataset generated by OpinionConv.}
\end{table}

\textbf{Conversation Template ID: 2}

\begin{table}[H]
\centering
\small

\begin{tabular}{@{}p{3cm}p{8.75cm}@{}}
\toprule
\bfseries Pair & \bfseries Example \\
\midrule
Deny--Switch Product &
{\bfseries C:} What I know about its screen, these phones, with their tiny screens and non-adjustable fonts, were just too small to deal with. \\
& \textcolor{salesassistantblue}{{\bfseries S:} If screens is important for you, we can offer this phone: Samsung Galaxy S, with bigger screen and better battery, it's just too hard to pass up.} \\
\midrule
Deny--Switch Feature &
{\bfseries C:} Yes! Screen plays a key role for me. I was told by one of my friends that when he has LTE service on, speed is insane. \\
& \textcolor{salesassistantblue}{{\bfseries S:} I can see what you’re saying but I disagree with you and beside that, the OS and its features are really easy to use.} \\
\midrule
Request--Inform &
{\bfseries C:} Ah, Ok! I’d be very interested to know your views on its battery. \\
& \textcolor{salesassistantblue}{{\bfseries S:} The battery life seems to be pretty good.} \\
\bottomrule
\end{tabular}
\caption{A dialogue example of conversation template (ID: 2) in dataset generated by OpinionConv.}
\end{table}

\newpage
\textbf{Conversation Template ID: 3}

\begin{table}[H]
\centering
\small

\begin{tabular}{@{}p{3cm}p{8.75cm}@{}}
\toprule
\bfseries Pair & \bfseries Example \\
\midrule
Deny--Switch Product &
{\bfseries C:} I was told by one of my friends about its camera that is below average quality for a new phone, and there is no LED flash. \\
& \textcolor{salesassistantblue}{{\bfseries S:} If camera is a crucial feature for you, we have this phone: LG G2, Camera takes great pictures and the video has good quality.} \\
\midrule
Deny--Switch Feature &
{\bfseries C:} Yes! camera plays a key role for me! What I know about its apps is that some of these useless apps take up a ridiculous amount of memory and automatically starts running in the background, whether you want it to or not. \\
& \textcolor{salesassistantblue}{{\bfseries S:} I’m sorry but I don’t think so, because you can decrease the memory usage of the apps and I would also mention something about the feature of this phone. If you want a nice, well made, feature rich smartphone get this one.} \\
\midrule
Request--Inform &
{\bfseries C:} Ah! I see! What is your opinion about its hardware? \\
& \textcolor{salesassistantblue}{{\bfseries S:} I bought this phone for myself and even with its one year old dated hardware, it still runs as fast as the newest android phone, because the company cares and has complete control over its OS so that it can be optimized the high extent.} \\
\bottomrule
\end{tabular}
\caption{A dialogue example of conversation template (ID: 3) in dataset generated by OpinionConv. The sales assistant expresses opinion in an argument for the Deny--Switch Feature pair.}
\end{table}

\textbf{Conversation Template ID: 4}

\begin{table}[H]
\centering
\small

\begin{tabular}{@{}p{3cm}p{8.75cm}@{}}
\toprule
\bfseries Pair & \bfseries Example \\
\midrule
Deny--Disagreement &
{\bfseries C:} I heard about its camera that its focus speed is quite slow, and the video does not appear to reliably auto focus without tapping the screen. \\
& \textcolor{salesassistantblue}{{\bfseries S:} Let me disagree with you, because this camera takes pretty sharp and colourful pix with its 8 megapixel camera and 5 megapixel front facing camera, HD video recording is also available.} \\
\midrule
Request--Inform &
{\bfseries C:} All right! Can you give me your thoughts on its screen size? \\
& \textcolor{salesassistantblue}{{\bfseries S:} The screen size is convenient for texting and reading documents or watching videos.} \\
\midrule
Search--Warning &
{\bfseries C:} I was wondering if you have this phone: Samsung Galaxy Alpha, it might be a good alternative because I've heard about its design that is really nice, handy and look attractive. \\
& \textcolor{salesassistantblue}{{\bfseries S:} Yes, this phone can also be a good choice but I should say about the signal of this phone that you probably get zero signal hardly in some places.} \\
\bottomrule
\end{tabular}
\caption{A dialogue example of conversation template (ID: 4) in dataset generated by OpinionConv.}
\end{table}

\newpage
\textbf{Conversation Template ID: 5}

\begin{table}[H]
\centering
\small

\begin{tabular}{@{}p{3cm}p{8.75cm}@{}}
\toprule
\bfseries Pair & \bfseries Example \\
\midrule
Request--Inform &
{\bfseries C:} I’d like to know your views on its features. \\
& \textcolor{salesassistantblue}{{\bfseries S:} They provide some new features that cause better integration for the Android OS.} \\
\midrule
Search--Warning &
{\bfseries C:} I was told by one of my friends about this phone: Samsung Galaxy S6 and its camera quality that one of his main reasons upgrading from a Galaxy S5 which he loved dearly to an S6 was because of the camera quality. \\
& \textcolor{salesassistantblue}{{\bfseries S:} Yes, That's for sure. This phone is also a good choice. However, about the screen of this phone I should say that it is not shatter proof.} \\
\midrule
Deny--Disagreement &
{\bfseries C:} Ah, Ok! What I know about its battery life of this phone is that it's not replaceable. \\
& \textcolor{salesassistantblue}{{\bfseries S:} No, it's not true, because one nice thing is that the batteries are user replaceable, inexpensive and readily available.} \\
\bottomrule
\end{tabular}
\caption{A dialogue example of conversation template (ID: 5) in dataset generated by OpinionConv.}
\end{table}

\textbf{Conversation Template ID: 6}

\begin{table}[H]
\centering
\small

\begin{tabular}{@{}p{3cm}p{8.75cm}@{}}
\toprule
\bfseries Pair & \bfseries Example \\
\midrule
Deny--Switch Feature &
{\bfseries C:} What I know about its signal is that it cuts out quite a bit where there's no signal at all. \\
& \textcolor{salesassistantblue}{{\bfseries S:} I’m sorry but I don’t think so. You receive signal properly with this phone and I would mention something about the design of this phone that this is a big size phone and with simple very efficient design.} \\
\midrule
Request--Inform &
{\bfseries C:} Can you give me your thoughts on its screen? \\
& \textcolor{salesassistantblue}{{\bfseries S:} The screen is clear and sharp, and it suits my needs just fine.} \\
\midrule
Search--Agreement &
{\bfseries C:} I was wondering if you have this phone: LG G Style, it might be a good choice because as far as I know it has a large screen and also long battery life. \\
& \textcolor{salesassistantblue}{{\bfseries S:} Yes, I agree. This phone is also a good choice. It's awesome how the phone has a split screen option.} \\
\midrule
Request--Inform &
{\bfseries C:} What do you think about its features? \\
& \textcolor{salesassistantblue}{{\bfseries S:} I would have loved a better quality camera, but all the other tech features at this price is simply awesome.} \\
\bottomrule
\end{tabular}
\caption{A dialogue example of Conversation template (ID: 6) in dataset generated by OpinionConv.}
\end{table}

\newpage
\textbf{Conversation Template ID: 7}

\begin{table}[H]
\centering
\small

\begin{tabular}{@{}p{3cm}p{8.75cm}@{}}
\toprule
\bfseries Pair & \bfseries Example \\
\midrule
Deny--Switch Feature &
{\bfseries C:} I heard about the camera of this phone that unfortunately, it is not of the same quality as many other phones even with less price. \\
& \textcolor{salesassistantblue}{{\bfseries S:}  I can understand what you’re saying but I disagree with you on its camera because it is able to take high quality pictures and even I can tell you about the features of this phone that has all the great features of the Galaxy S3, along with a bigger screen, stylus and Factory loaded Android Jelly Bean OS.} \\
\midrule
Request--Inform &
{\bfseries C:} Could you tell me your opinion on its size? \\
& \textcolor{salesassistantblue}{{\bfseries S:} t has a nice size for someone who doesn't want to have a too big smartphone.} \\
\midrule
Search--Switch Feature &
{\bfseries C:} I was told by one of my friends about this phone: BlackBerry Q10 that its keyboard is great, screen is clear, and the battery life is good, not outstanding, but good. \\
& \textcolor{salesassistantblue}{{\bfseries S:} Yes, That's for sure. This phone is also a good choice. It has also some useful features for its camera.} \\
\midrule
Request--Inform &
{\bfseries C:} What do you think about its resolution? \\
& \textcolor{salesassistantblue}{{\bfseries S:} It has a great resolution, a perfect size and excellent color reproduction.} \\
\bottomrule
\end{tabular}
\caption{A dialogue example of conversation template (ID: 7) in dataset generated by OpinionConv.}
\end{table}

\textbf{Conversation Template ID: 8}

\begin{table}[H]
\centering
\small

\begin{tabular}{@{}p{3cm}p{8.75cm}@{}}
\toprule
\bfseries Pair & \bfseries Example \\
\midrule
Request--Inform &
{\bfseries C:} I’d be very interested to know your views on its screen. \\
& \textcolor{salesassistantblue}{{\bfseries S:} For this price, the screen and resolution are both good.} \\
\midrule
Deny--Switch Product &
{\bfseries C:} But I heard about its camera that my friend was a bit annoyed by the quality of the pictures taken by the camera. \\
& \textcolor{salesassistantblue}{{\bfseries S:} If camera is a crucial feature for you, we have this phone: LG G3. The camera with 16mp takes good quality pictures.} \\
\midrule
Request--Inform &
{\bfseries C:} Ah! Ok! What is your opinion about its screen? \\
& \textcolor{salesassistantblue}{{\bfseries S:} The screen is beautiful and big, fast, smooth and bright.} \\
\bottomrule
\end{tabular}
\caption{A dialogue example of conversation template (ID: 8) in dataset generated by OpinionConv.}
\end{table}

\newpage
\textbf{Conversation Template ID: 9}

\begin{table}[H]
\centering
\small

\begin{tabular}{@{}p{3cm}p{8.75cm}@{}}
\toprule
\bfseries Pair & \bfseries Example \\
\midrule
Search--Agreement &
{\bfseries C:} I was wondering if you have this phone: Samsung Galaxy S4. I was told by one of my friends  that is a nice and reliable smartphone and is easy to use with an SD card. \\
& \textcolor{salesassistantblue}{{\bfseries S:} Yes, That's exactly what I know about this phone. So, this is also a good choice. It has also excellent sound quality.} \\
\midrule
Request--Inform &
{\bfseries C:} Ok! Great! May I know your opinion on its speakers? \\
& \textcolor{salesassistantblue}{{\bfseries S:} It has stereo speakers with surround sound.} \\
\bottomrule
\end{tabular}
\caption{A dialogue example of conversation template (ID: 9) in dataset generated by OpinionConv.}
\end{table}

\textbf{Conversation Template ID: 10}

\begin{table}[H]
\centering
\small

\begin{tabular}{@{}p{3cm}p{8.75cm}@{}}
\toprule
\bfseries Pair & \bfseries Example \\
\midrule
Search--Switch Feature &
{\bfseries C:} I wanted to know if you have this phone: LG G5, it might be a good choice because this has a reasonable price with a big screen. \\
& \textcolor{salesassistantblue}{{\bfseries S:} Yes, that's for sure. This should be a good choice for you.} \\
\midrule
Request--Inform &
{\bfseries C:} Ok! Good!Do you have any particular views on its features? \\
& \textcolor{salesassistantblue}{{\bfseries S:} This phone has all the features you need for a phone.} \\
\bottomrule
\end{tabular}
\caption{A dialogue example of conversation template (ID: 10) in dataset generated by OpinionConv.}
\end{table}

\textbf{Conversation Template ID: 11}

\begin{table}[H]
\centering
\small

\begin{tabular}{@{}p{3cm}p{8.75cm}@{}}
\toprule
\bfseries Pair & \bfseries Example \\
\midrule
Request--Inform &
{\bfseries C:} I was wondering if you have this phone: HTC One, it can be a good choice for me because I heard that the camera of the phone works great. \\
& \textcolor{salesassistantblue}{{\bfseries S:} Yes, I agree with you but I should say that it doesn't have many additional features that the other phones have in the same price range.} \\
\midrule
Deny--Disagreement &
{\bfseries C:} But I don't need the additional features. Could you tell me your opinion on its design? \\
& \textcolor{salesassistantblue}{{\bfseries S:} You would love the design and it fits applications.} \\
\midrule
Request--Inform &
{\bfseries C:} Ah! I see! What is your opinion about its hardware? \\
& \textcolor{salesassistantblue}{{\bfseries S:} I bought this phone for myself and even with its one year old dated hardware, it still runs as fast as the newest android phone, because the company cares and has complete control over its OS so that it can be optimized the high extent.} \\
\bottomrule
\end{tabular}
\caption{A dialogue example of conversation template (ID: 11) in dataset generated by OpinionConv.}
\end{table}

\textbf{Conversation Template ID: 12}

\begin{table}[H]
\centering
\small

\begin{tabular}{@{}p{3cm}p{8.75cm}@{}}
\toprule
\bfseries Pair & \bfseries Example \\
\midrule
Search--Switch Feature &
{\bfseries C:} I wanted to know if you have this phone: Microsoft Lumia, because I heard that it has a simple interface; easy to use. \\
& \textcolor{salesassistantblue}{{\bfseries S:} Yes, it's true. This is a good choice. It has also excellent sound quality.} \\
\midrule
Search--Switch Product &
{\bfseries C:} Ah! Having a good camera is important for me! \\
& \textcolor{salesassistantblue}{{\bfseries S:} Okay! So, I can offer you this one: LG Optimus with a really great camera.} \\
\midrule
Request--Inform &
{\bfseries C:} In your honest opinion, how is its screen? \\
& \textcolor{salesassistantblue}{{\bfseries S:}  I have bought this phone for myself and the only thing that was holding me back from upgrading to another phone was how large the screen of this phone is.} \\
\bottomrule
\end{tabular}
\caption{A dialogue example of conversation template (ID: 12) in dataset generated by OpinionConv.}
\end{table}

\textbf{Conversation Template ID: 13}

\begin{table}[H]
\centering
\small

\begin{tabular}{@{}p{3cm}p{8.75cm}@{}}
\toprule
\bfseries Pair & \bfseries Example \\
\midrule
Request--Inform &
{\bfseries C:} May I know your opinion on its speakers? \\
& \textcolor{salesassistantblue}{{\bfseries S:} The speakers are loud and clear for music.} \\
\midrule
Deny--Switch Feature &
{\bfseries C:} I heard about its battery that loses its charge in just a few hours. \\
& \textcolor{salesassistantblue}{{\bfseries S:} I’m sorry but let me disagree with you, because the battery lasts for up to 6 hours with the display on and even I can tell you that one other cool feature is a dedicated "custom" button that you can assign/ reassign to activate any feature or app or widget.} \\
\midrule
Search--Warning &
{\bfseries C:} I wanted to ask if you have this phone: Samsung Galaxy S4, it might be a good choice for me because I heard this phone is far superior in quality and function, not even close. \\
& \textcolor{salesassistantblue}{{\bfseries S:} Yes, That's so true. This phone can be also a good alternative but I should say that this phone has very limited space/ memory for apps.} \\
\midrule
Request--Inform &
{\bfseries C:} I see! I’d like to know your views on its size. \\
& \textcolor{salesassistantblue}{{\bfseries S:} Just the right size and it doesn't feel like a tablet in your pocket.} \\
\bottomrule
\end{tabular}
\caption{A dialogue example of conversation template (ID: 13) in dataset generated by OpinionConv.}
\end{table}

\newpage
\textbf{Conversation Template ID: 14}

\begin{table}[H]
\centering
\small

\begin{tabular}{@{}p{3cm}p{8.75cm}@{}}
\toprule
\bfseries Pair & \bfseries Example \\
\midrule
Deny--Switch Item &
{\bfseries C:} I was told by my friend that battery heating errors appear quite unusually ob the screen. \\
& \textcolor{salesassistantblue}{{\bfseries S:} If battery is a crucial feature for you, we have this phone: Motorola G The battery life seems good.} \\
\midrule
Request--Inform &
{\bfseries C:} Great! I’d be interested to know your views on its camera. \\
& \textcolor{salesassistantblue}{{\bfseries S:} The 8-megapixel camera is awesome and takes great pictures.
8-megapixel camera} \\
\midrule
Search--Switch Feature &
{\bfseries C:} I wanted to know if you have this phone: Samsung S6 because the phone size is thicker, lighter and narrower than the iPhone, hence easier to hold onto. \\
& \textcolor{salesassistantblue}{{\bfseries S:} Yes, I agree. It has also a great resolution and excellent color reproduction.} \\
\midrule
Request--Inform &
{\bfseries C:} Can you tell me your thoughts about its screen? \\
& \textcolor{salesassistantblue}{{\bfseries S:} This phone has a great screen, 1080P, very bright and true colors.} \\
\bottomrule
\end{tabular}
\caption{A dialogue example of conversation template (ID: 14) in dataset generated by OpinionConv.}
\end{table}

\newpage
\section{Evaluation Questionnaire for Study 1}
(form starts next page)

\includepdf[pages=-,scale=.9]{sigir23-opinionConv-figures/human-evaluation-questionnaire-study1.pdf}

\newpage
\section{Evaluation Questionnaire for Study 2}
(form starts next page)

\includepdf[pages=-,scale=.9]{sigir23-opinionConv-figures/human-evaluation-questionnaire-study2.pdf}

\newpage
\section{Feature-Value Pairs}

\begin{table}[H]
\centering
\begin{tabular}{@{}ll@{}}
\toprule
\textbf{Feature} & \textbf{Value}                     \\
\midrule
Brand           & Apple, Samsung, LG, Motorola, etc. \\
OS              & ios, android, windows              \\
Memory          & 2 GB, 4 GB, 8 GB, etc              \\
Color           & black, white, red, etc.            \\
\bottomrule
\end{tabular}
\caption{Feature-value pairs for generating information search dialogues}
\end{table}

\section{Human Evaluation Results for Study 2}

\begin{table}[H]
\centering
\begin{tabular}{lll|ll|ll|ll}
\toprule
& \multicolumn{2}{c}{Definitely yes} & \multicolumn{2}{c}{Rather yes} & \multicolumn{2}{c}{Rather  not} & \multicolumn{2}{c}{Definitely not} \\
\midrule
& \multicolumn{1}{c}{F} & \multicolumn{1}{c}{M} & \multicolumn{1}{c}{F} & \multicolumn{1}{c}{M} & \multicolumn{1}{c}{F} & \multicolumn{1}{c}{M} & \multicolumn{1}{c}{F} & \multicolumn{1}{c}{M} \\
\midrule
Q1 & 17.47\%  & 8.4\% & 37.9\% & 14.4\% & 13.2\% & 6.6\% & 1.8\% & - \\
\midrule
Q2 & 10.8\% & 1.8\% & 31.9\% & 16.3\% & 21.7\% & 7.8\% & 6.0\% & 3.6\% \\
\midrule
Q3 & 10.2\% & 3.0\% & 36.7\% & 16.3\% & 16.7\% & 10.2\% & 6.6\% & - \\
\midrule
Q4 & 12.6\% & 5.4\% & 42.8\% & 16.9\% & 13.2\% & 7.2\% & 1.8\% & - \\
\midrule
Q5 & 9.6\% & 2.4\% & 29.5\% & 13.2\% & 24.7\% & 12.0\% & 6.6\% & 1.8\% \\
\midrule
Q6 & 9.6\% & 4.2\% & 35.5\% & 15.0\% & 22.3\% & 9.6\% & 3.0\% & 0.6\% \\
\bottomrule
\end{tabular}
\caption{Human evaluation results for study 2 separated by gender}
\end{table}

\newpage
\section{ChatGPT vs YouChat}

\textbf{ChatGPT response:}
As shown below, ChatGPT doesn't have any personal thoughts or opinions on this topic.
\newline

\includegraphics[scale=.3]{sigir23-opinionConv-figures/image_ChatGPT.png}

\textbf{YouChat response:}
We can receive an answer/ opinion from YouChat when we ask the same question. However, the next response rejects the previous one regrading the quality of battery life of android smartphones.
\newline

\includegraphics[scale=.55]{sigir23-opinionConv-figures/image_YouChat.png}

\includegraphics[scale=.55]{sigir23-opinionConv-figures/image_YouChat_1.png}
